# Supplementary material for: FedHiSyn: A Hierarchical Synchronous Federated Learning Framework for Resource and Data Heterogeneity
Source: arXiv:2206.10546 source file (2022-06-21)
Supplement: Supplementary file 1 [file appendix.tex]

\onecolumn
\section{Appendix}

\subsection{Proof of Lemma 5.1}

The parameters uploaded by device $i$ will be trained on devices $\Omega_i$, and the parameters after the training of the $j$ th device are denoted as $\mathcal{W}_i^j$, $j \in \Omega_i$.We assume that the learning rate $\eta$ remains the same during the training of communication between devices.
\begin{align}
\mathcal{W}_i^{j+1}  &= \mathcal{W}_i^{j} -    \eta F_j(\mathcal{W}_i^{rj},\xi_i^j)   
\end{align}
thus, 
\begin{align}
\mathcal{W}_i^{1} -  \mathcal{W}_i^{\left\|\Omega_i\right\|}&= \mathcal{W}_i^{1} - \mathcal{W}_i^{2},\ldots, +\mathcal{W}_i^{\left\|\Omega_i\right\|-1} -  \mathcal{W}_i^{\left\|\Omega_i\right\|} \\
&= \eta F_i(\mathcal{W}_i^{1},\xi_t^1),\ldots, + \eta F_i(\mathcal{W}_i^{\left\|\Omega_i\right\|-1},\xi_t^{\left\|\Omega_i\right\|-1})\\
&= \eta \sum_{j=1}^{\left\|\Omega_i\right\|-1} F_i(j_i^{r},\xi_i^j)
\end{align}  
With Definition 5.1, and Assumption 5.4
\begin{align}
\nabla \tilde{F}_i(\mathcal{W}) &= \frac{\mathcal{W}_{initial} - \mathcal{W}_{trained}}{\eta}\\
& =\sum_{j=1}^{\left\|\Omega_i\right\|-1} F_i(\mathcal{W}_i^{j},\xi_j^2)\\
&  \leq \sum_{j=1}^{\left\|\Omega_i\right\|-1} G^2 \\
&=(\left\|\Omega_i\right\|-1) G^2
\end{align}

\subsection{Convergence description with partial participation }
In the work\cite{DBLP:conf/iclr/LiHYWZ20}, in order to prove the convergence for partial device participation,  Assumption A.1 is made. Assumption A.1 assumes the $Q$ indices are selected from the distribution $p_i$ independently and with replacement. The aggregation step is simply averaging. 

\textbf{Assumption A.1.}
	Assume $\mathcal{S}_r$ contains a subset of $J$ indices randomly selected {with replacement} according to the sampling probabilities $p_1, \cdots , p_C$. The aggregation step of \texttt{FedAvg} performs
	$\mathcal{W}_{r}  = \frac{1}{J} \sum_{j \in \mathcal{S} } \mathcal{W}_{i}^r $.

We consider the simple case where partial devices will participate in training. According to the conclusion of work\cite{DBLP:conf/iclr/LiHYWZ20}, with 	Assumptions 5.1, 5.2, A.1, Definition 5.2 and Lemma 5.1 we can get Theorem A.1 of FedHiSyn.
\textbf{Theorem A.1.}	
	In FedHiSyn, Eq. (9) supports the Assumption A.1. Let  $L, \mu, \sigma_k, G$ be defined therein. Let $\kappa, \gamma$, $\eta_t$, and $B$ be defined in Theorem 5.1.
	define $C =  \frac{4}{K} E^2G^2$.
	Then 
	\begin{equation}	
	\mathbb{E}\left[ F(\mathcal{W}_R)\right] - F^* 
	\: \leq \: 
	\frac{2\kappa}{\gamma + R} \left( \frac{B + C}{\mu} + 2L \|\mathcal{W}_0 - \mathcal{W}^*\|^2 \right).
	\end{equation}
The detailed proof of Theorem A.1  refer to the works \cite{DBLP:conf/iclr/LiHYWZ20}.
As $R$ increases, the right side of the equation approaches 0, so FedHiSyn can converge to the global optimum when partial devices  participate in training.
